# Supplementary material for: Broken Neural Scaling Laws
Source: arXiv:2210.14891 source file (2023-07-24)
Supplement: Supplementary file 1 [file sec_appendix.tex]

\section{Appendix}
You may include other additional sections here.

\section{Experimental details of \ref{section:Inflection_Points}}
We perform an extensive set of experiments to model and extrapolate the scaling behavior for the 4-digit arithmetic addition task with respect to the training dataset size.We set the batch size equal to the training dataset size. We do not use dropout or a learning rate decay here. For our experiments we train the transformer model using the following set of hyperparameters:
\begin{table}[hbt!]
    \centering
    \begin{tabular}{c|c}
         Model Embedding size & 128 \\
         Number of heads & 2 \\
         Number of layers & 1 \\
         Learning rate & 0.0001\\
         Dropout Probability & 0.0\\
         Test set size & 1000\\
    \end{tabular}
    \caption{Hyperparameters for 4-digit addition task}
    \label{tab:my_label}
\end{table}

\section{All Tables and Plots on the Scaling Laws Benchmark of \citet{Alabdulmohsi2022revisiting}}
\label{all_scaling_laws}

\subsection{Table of Extrapolations}

\FloatBarrier

\begin{table}
\tiny
\setlength\tabcolsep{3.1pt} 
\begin{tabular}
%{p{.02\textwidth}p{.165\textwidth}p{.095\textwidth}p{.01\textwidth}p{.01\textwidth}p{.099\textwidth}p{.099\textwidth}p{.099\textwidth}p{.099\textwidth}p{.099\textwidth}}
{p{.021\textwidth}p{.165\textwidth}p{.111\textwidth}p{.028\textwidth}p{.022\textwidth}p{.099\textwidth}p{.099\textwidth}p{.099\textwidth}p{.099\textwidth}p{.099\textwidth}}
%\begin{tabular}{llllrrrrrrrrrrrrl}
Domain & \hspace{.9cm}Task & Model & Train Points & Test Points & M1 \downarrow & M2 \downarrow & M3 \downarrow & M4 \downarrow & BNSL \downarrow \\
\hline
BB & date understanding, 1-shot & 2.62e+8 Param & 19 & 24 & 3.19e-2 ± 9.6e-4 & 3.09e-2 ± 9.2e-4 & \bfseries 4.67e-3 ± 1.4e-4 & 1.49e-2 ± 5.9e-4 & 4.96e-3 ± 4.8e-5 \\
BB & date understanding, 2-shot & 2.62e+8 Param & 19 & 24 & 2.86e-2 ± 6.2e-4 & 2.44e-2 ± 5.6e-4 & 4.83e-3 ± 4.1e-4 & 1.58e-2 ± 5.0e-4 & \bfseries 2.55e-3 ± 6.2e-4 \\
BB & linguistic mappings, 1-shot & 2.62e+8 Param & 19 & 24 & 1.66e-2 ± 5.5e-4 & \bfseries 1.41e-2 ± 4.7e-4 & 1.66e-2 ± 5.5e-4 & 1.57e-2 ± 4.8e-4 & 2.22e-2 ± 8.2e-4 \\
BB & linguistic mappings, 2-shot & 2.62e+8 Param & 19 & 24 & 1.70e-2 ± 6.5e-4 & 1.30e-2 ± 5.4e-4 & 1.70e-2 ± 6.5e-4 & 9.25e-3 ± 5.1e-4 & \bfseries 8.09e-3 ± 5.1e-4 \\
BB & mult data wrangling, 1-shot & 2.62e+8 Param & 19 & 24 & 1.07e-2 ± 1.0e-3 & 6.71e-3 ± 7.6e-4 & 1.07e-2 ± 1.0e-3 & 8.27e-3 ± 8.4e-4 & \bfseries 6.17e-3 ± 8.4e-4 \\
BB & mult data wrangling, 2-shot & 2.62e+8 Param & 19 & 24 & 1.57e-2 ± 1.5e-3 & 7.22e-3 ± 8.9e-4 & 1.57e-2 ± 1.5e-3 & \bfseries 5.01e-3 ± 5.0e-4 & 5.45e-3 ± 9.2e-4 \\
BB & qa wikidata, 1-shot & 2.62e+8 Param & 19 & 24 & \bfseries 4.27e-3 ± 8.9e-4 & 5.14e-3 ± 5.3e-4 & 4.27e-3 ± 8.9e-4 & 5.05e-3 ± 5.6e-4 & 4.34e-3 ± 6.1e-4 \\
BB & qa wikidata, 2-shot & 2.62e+8 Param & 19 & 24 & 4.39e-3 ± 7.0e-4 & 7.35e-3 ± 6.1e-4 & 4.39e-3 ± 7.0e-4 & 7.12e-3 ± 6.0e-4 & \bfseries 4.20e-3 ± 6.0e-4 \\
BB & unit conversion, 1-shot & 2.62e+8 Param & 19 & 24 & 8.30e-3 ± 4.4e-4 & 6.77e-3 ± 4.0e-4 & \bfseries 1.48e-3 ± 2.7e-4 & 2.32e-3 ± 2.3e-4 & 6.32e-3 ± 2.5e-4 \\
BB & unit conversion, 2-shot & 2.62e+8 Param & 19 & 24 & 1.07e-2 ± 4.4e-4 & 9.15e-3 ± 4.7e-4 & 7.50e-3 ± 5.5e-4 & \bfseries 2.83e-3 ± 4.8e-4 & 5.21e-3 ± 5.2e-4 \\
IC & Birds 200 10-shot & BiT/101/3 & 57 & 107 & 9.13e-2 ± 2.8e-3 & 9.13e-2 ± 2.8e-3 & 9.13e-2 ± 2.8e-3 & 2.49e-2 ± 1.2e-3 & \bfseries 3.79e-3 ± 1.1e-3 \\
IC & Birds 200 10-shot & BiT/50/1 & 70 & 469 & 6.88e-2 ± 7.5e-4 & 6.88e-2 ± 7.5e-4 & 5.24e-2 ± 6.2e-4 & 2.48e-2 ± 5.1e-4 & \bfseries 4.96e-3 ± 3.9e-4 \\
IC & Birds 200 10-shot & MiX/B/16 & 69 & 383 & 9.15e-2 ± 1.1e-3 & 9.15e-2 ± 1.1e-3 & 3.95e-2 ± 7.0e-4 & 4.14e-2 ± 7.8e-4 & \bfseries 9.98e-3 ± 7.0e-4 \\
IC & Birds 200 10-shot & MiX/L/16 & 63 & 211 & 5.51e-2 ± 1.4e-3 & 5.51e-2 ± 1.4e-3 & 5.51e-2 ± 1.4e-3 & 4.59e-2 ± 1.6e-3 & \bfseries 8.41e-3 ± 1.3e-3 \\
IC & Birds 200 10-shot & ViT/B/16 & 65 & 316 & 6.77e-2 ± 1.1e-3 & 6.77e-2 ± 1.1e-3 & 3.52e-2 ± 8.1e-4 & 1.87e-2 ± 7.2e-4 & \bfseries 9.81e-3 ± 8.1e-4 \\
IC & Birds 200 10-shot & ViT/S/16 & 54 & 133 & 3.95e-2 ± 1.2e-3 & 3.95e-2 ± 1.2e-3 & 3.74e-2 ± 1.1e-3 & \bfseries 9.81e-3 ± 5.4e-4 & 1.51e-2 ± 8.4e-4 \\
IC & Birds 200 25-shot & BiT/101/3 & 53 & 78 & 9.41e-2 ± 3.2e-3 & 9.41e-2 ± 3.2e-3 & 9.41e-2 ± 3.2e-3 & 5.09e-2 ± 1.8e-3 & \bfseries 7.24e-3 ± 1.6e-3 \\
IC & Birds 200 25-shot & BiT/50/1 & 69 & 452 & 1.10e-1 ± 1.0e-3 & 7.29e-2 ± 8.0e-4 & 1.52e-2 ± 4.9e-4 & 1.63e-2 ± 5.1e-4 & \bfseries 8.00e-3 ± 6.1e-4 \\
IC & Birds 200 25-shot & MiX/B/16 & 67 & 293 & 1.40e-1 ± 1.9e-3 & 1.40e-1 ± 1.9e-3 & 6.93e-2 ± 1.2e-3 & 1.85e-2 ± 6.3e-4 & \bfseries 5.02e-3 ± 6.2e-4 \\
IC & Birds 200 25-shot & MiX/L/16 & 63 & 196 & 1.12e-1 ± 2.0e-3 & 1.12e-1 ± 2.0e-3 & 1.12e-1 ± 2.0e-3 & 4.88e-2 ± 1.8e-3 & \bfseries 1.05e-2 ± 1.7e-3 \\
IC & Birds 200 25-shot & ViT/B/16 & 64 & 271 & 9.02e-2 ± 1.6e-3 & 9.02e-2 ± 1.6e-3 & 3.75e-2 ± 1.0e-3 & 1.52e-2 ± 5.8e-4 & \bfseries 5.87e-3 ± 6.1e-4 \\
IC & Birds 200 25-shot & ViT/S/16 & 51 & 100 & 5.06e-2 ± 1.4e-3 & 5.06e-2 ± 1.4e-3 & 4.96e-2 ± 1.4e-3 & 3.28e-2 ± 1.1e-3 & \bfseries 1.21e-2 ± 8.5e-4 \\
IC & Birds 200 5-shot & BiT/101/3 & 62 & 180 & 8.17e-2 ± 2.0e-3 & 8.17e-2 ± 2.0e-3 & 8.17e-2 ± 2.0e-3 & 3.00e-2 ± 1.2e-3 & \bfseries 6.08e-3 ± 1.1e-3 \\
IC & Birds 200 5-shot & BiT/50/1 & 71 & 517 & 5.44e-2 ± 5.6e-4 & 5.44e-2 ± 5.6e-4 & 5.44e-2 ± 5.6e-4 & 2.63e-2 ± 5.4e-4 & \bfseries 5.79e-3 ± 3.7e-4 \\
IC & Birds 200 5-shot & MiX/B/16 & 71 & 494 & 8.27e-2 ± 1.0e-3 & 8.27e-2 ± 1.0e-3 & 5.49e-2 ± 7.8e-4 & 1.86e-2 ± 5.0e-4 & \bfseries 5.74e-3 ± 4.7e-4 \\
IC & Birds 200 5-shot & MiX/L/16 & 67 & 326 & 5.68e-2 ± 1.4e-3 & 5.68e-2 ± 1.4e-3 & 5.68e-2 ± 1.4e-3 & 2.65e-2 ± 9.0e-4 & \bfseries 5.06e-3 ± 6.4e-4 \\
IC & Birds 200 5-shot & ViT/B/16 & 65 & 284 & 3.40e-2 ± 8.9e-4 & 3.40e-2 ± 8.9e-4 & 3.40e-2 ± 8.9e-4 & 1.26e-2 ± 5.3e-4 & \bfseries 6.32e-3 ± 5.8e-4 \\
IC & Birds 200 5-shot & ViT/S/16 & 57 & 150 & 2.75e-2 ± 7.9e-4 & 2.75e-2 ± 7.9e-4 & 2.75e-2 ± 7.9e-4 & 1.56e-2 ± 5.9e-4 & \bfseries 6.93e-3 ± 4.8e-4 \\
IC & CIFAR-100 10-shot & BiT/101/3 & 47 & 60 & 8.57e-2 ± 3.8e-3 & 8.57e-2 ± 3.8e-3 & 8.25e-2 ± 3.7e-3 & 9.28e-2 ± 3.9e-3 & \bfseries 1.53e-2 ± 2.9e-3 \\
IC & CIFAR-100 10-shot & BiT/50/1 & 62 & 192 & 7.44e-2 ± 1.5e-3 & 1.24e-2 ± 5.8e-4 & 2.08e-2 ± 7.2e-4 & 1.23e-2 ± 5.7e-4 & \bfseries 9.74e-3 ± 7.1e-4 \\
IC & CIFAR-100 10-shot & MiX/B/16 & 65 & 248 & 8.77e-2 ± 1.9e-3 & 8.77e-2 ± 1.9e-3 & 2.71e-2 ± 1.2e-3 & 2.60e-2 ± 1.2e-3 & \bfseries 8.61e-3 ± 9.5e-4 \\
IC & CIFAR-100 10-shot & MiX/L/16 & 67 & 313 & 1.05e-1 ± 3.1e-3 & 1.05e-1 ± 3.1e-3 & 4.85e-2 ± 2.6e-3 & 4.76e-2 ± 1.7e-3 & \bfseries 1.55e-2 ± 1.6e-3 \\
IC & CIFAR-100 10-shot & ViT/B/16 & 67 & 354 & 8.98e-2 ± 2.0e-3 & 8.98e-2 ± 2.0e-3 & 8.98e-2 ± 2.0e-3 & 5.60e-2 ± 1.8e-3 & \bfseries 1.73e-2 ± 1.8e-3 \\
IC & CIFAR-100 10-shot & ViT/S/16 & 67 & 450 & 6.84e-2 ± 1.1e-3 & 2.11e-2 ± 6.6e-4 & 3.35e-2 ± 8.6e-4 & 2.47e-2 ± 7.4e-4 & \bfseries 1.15e-2 ± 7.5e-4 \\
IC & CIFAR-100 25-shot & BiT/101/3 & 41 & 38 & 8.77e-2 ± 5.6e-3 & 8.77e-2 ± 5.6e-3 & 4.44e-2 ± 3.5e-3 & 4.29e-2 ± 3.4e-3 & \bfseries 9.32e-3 ± 3.0e-3 \\
IC & CIFAR-100 25-shot & BiT/50/1 & 55 & 109 & 7.31e-2 ± 2.0e-3 & 2.35e-2 ± 1.5e-3 & 3.65e-2 ± 1.8e-3 & 2.36e-2 ± 1.5e-3 & \bfseries 2.00e-2 ± 1.8e-3 \\
IC & CIFAR-100 25-shot & MiX/B/16 & 64 & 202 & 1.08e-1 ± 2.3e-3 & 4.75e-2 ± 1.6e-3 & 2.10e-2 ± 9.4e-4 & 2.08e-2 ± 9.3e-4 & \bfseries 8.15e-3 ± 1.1e-3 \\
IC & CIFAR-100 25-shot & MiX/L/16 & 62 & 185 & 9.79e-2 ± 2.2e-3 & 9.79e-2 ± 2.2e-3 & 3.67e-2 ± 1.7e-3 & 2.79e-2 ± 1.3e-3 & \bfseries 8.47e-3 ± 1.6e-3 \\
IC & CIFAR-100 25-shot & ViT/B/16 & 66 & 355 & 1.07e-1 ± 1.9e-3 & 1.07e-1 ± 1.9e-3 & 6.54e-2 ± 1.6e-3 & \bfseries 4.81e-2 ± 1.4e-3 & 1.20e-1 ± 1.4e-3 \\
IC & CIFAR-100 25-shot & ViT/S/16 & 66 & 416 & 8.03e-2 ± 1.2e-3 & 2.19e-2 ± 7.4e-4 & 3.13e-2 ± 8.4e-4 & 2.19e-2 ± 7.0e-4 & \bfseries 1.34e-2 ± 8.5e-4 \\
IC & CIFAR-100 5-shot & BiT/101/3 & 47 & 59 & 5.94e-2 ± 3.2e-3 & 5.94e-2 ± 3.2e-3 & 5.94e-2 ± 3.2e-3 & 4.57e-2 ± 2.8e-3 & \bfseries 1.58e-2 ± 2.6e-3 \\
IC & CIFAR-100 5-shot & BiT/50/1 & 57 & 98 & 4.87e-2 ± 1.3e-3 & 4.87e-2 ± 1.3e-3 & \bfseries 1.69e-2 ± 8.8e-4 & 4.91e-2 ± 1.3e-3 & 1.95e-2 ± 1.0e-3 \\
IC & CIFAR-100 5-shot & MiX/B/16 & 66 & 304 & 7.07e-2 ± 1.2e-3 & 7.07e-2 ± 1.2e-3 & 2.78e-2 ± 8.4e-4 & 2.05e-2 ± 7.4e-4 & \bfseries 6.77e-3 ± 6.3e-4 \\
IC & CIFAR-100 5-shot & MiX/L/16 & 67 & 312 & 7.06e-2 ± 1.6e-3 & 7.06e-2 ± 1.6e-3 & 4.17e-2 ± 1.4e-3 & 3.14e-2 ± 1.1e-3 & \bfseries 1.18e-2 ± 1.3e-3 \\
IC & CIFAR-100 5-shot & ViT/B/16 & 67 & 352 & 6.27e-2 ± 1.6e-3 & 6.27e-2 ± 1.6e-3 & 6.27e-2 ± 1.6e-3 & 5.11e-2 ± 1.4e-3 & \bfseries 1.19e-2 ± 1.2e-3 \\
IC & CIFAR-100 5-shot & ViT/S/16 & 70 & 710 & 6.93e-2 ± 1.2e-3 & \bfseries 2.84e-2 ± 8.2e-4 & 3.88e-2 ± 8.0e-4 & 3.09e-2 ± 7.5e-4 & 6.40e-2 ± 7.7e-4 \\
IC & Caltech101 10-shot & BiT/101/3 & 21 & 14 & 3.07e-1 ± 2.0e-2 & 3.07e-1 ± 2.0e-2 & 1.51e-1 ± 1.3e-2 & 3.54e-2 ± 6.3e-3 & \bfseries 6.42e-3 ± 5.8e-3 \\
IC & Caltech101 10-shot & BiT/50/1 & 33 & 16 & 3.29e-1 ± 1.6e-2 & 7.68e-2 ± 5.0e-3 & 1.13e-1 ± 6.0e-3 & 6.31e-2 ± 4.4e-3 & \bfseries 5.37e-3 ± 2.2e-3 \\
IC & Caltech101 10-shot & MiX/B/16 & 14 & 12 & 1.35e-1 ± 1.4e-2 & 1.35e-1 ± 1.4e-2 & 1.35e-1 ± 1.4e-2 & 2.11e-1 ± 1.7e-2 & \bfseries 3.72e-2 ± 9.7e-3 \\
IC & Caltech101 10-shot & MiX/L/16 & 12 & 11 & 1.25e-1 ± 1.3e-2 & 1.25e-1 ± 1.3e-2 & 1.25e-1 ± 1.3e-2 & 1.92e-1 ± 1.6e-2 & \bfseries 3.73e-2 ± 1.5e-2 \\
IC & Caltech101 10-shot & ViT/B/16 & 34 & 33 & 7.76e-2 ± 4.3e-3 & 7.76e-2 ± 4.3e-3 & 3.11e-2 ± 3.0e-3 & 5.54e-2 ± 4.3e-3 & \bfseries 1.67e-2 ± 5.4e-3 \\
IC & Caltech101 10-shot & ViT/S/16 & 43 & 55 & 1.95e-1 ± 6.0e-3 & 3.41e-2 ± 2.9e-3 & \bfseries 2.40e-2 ± 2.0e-3 & 3.95e-2 ± 3.1e-3 & 3.31e-2 ± 5.3e-3 \\
IC & Caltech101 25-shot & BiT/101/3 & 10 & 3 & 1.15e-1 ± 6.5e-3 & 1.15e-1 ± 6.5e-3 & 1.15e-1 ± 6.5e-3 & 5.23e-2 ± 2.7e-3 & \bfseries 1.13e-2 ± 8.0e-3 \\
IC & Caltech101 25-shot & BiT/50/1 & 28 & 16 & 3.60e-1 ± 1.9e-2 & 8.80e-2 ± 5.5e-3 & 1.43e-1 ± 7.6e-3 & 5.95e-2 ± 4.1e-3 & \bfseries 2.13e-3 ± 1.6e-3 \\
IC & Caltech101 25-shot & MiX/B/16 & 13 & 11 & 8.28e-2 ± 1.2e-2 & 8.28e-2 ± 1.2e-2 & 8.28e-2 ± 1.2e-2 & 1.74e-1 ± 1.7e-2 & \bfseries 2.83e-2 ± 1.3e-2 \\
IC & Caltech101 25-shot & MiX/L/16 & 12 & 12 & 9.66e-2 ± 1.0e-2 & 9.66e-2 ± 1.0e-2 & 9.66e-2 ± 1.0e-2 & 1.03e-1 ± 9.5e-3 & \bfseries 1.98e-2 ± 1.3e-2 \\
IC & Caltech101 25-shot & ViT/B/16 & 27 & 28 & 1.03e-1 ± 5.6e-3 & 3.33e-2 ± 2.5e-3 & 4.46e-2 ± 3.6e-3 & 4.24e-2 ± 3.6e-3 & \bfseries 6.37e-3 ± 5.4e-3 \\
IC & Caltech101 25-shot & ViT/S/16 & 41 & 54 & 1.77e-1 ± 5.4e-3 & 3.79e-2 ± 3.1e-3 & 2.80e-2 ± 1.8e-3 & \bfseries 2.35e-2 ± 2.3e-3 & 2.38e-2 ± 4.7e-3 \\
IC & Caltech101 5-shot & BiT/101/3 & 16 & 13 & 2.12e-1 ± 1.2e-2 & 2.12e-1 ± 1.2e-2 & 2.12e-1 ± 1.2e-2 & 8.82e-2 ± 5.0e-3 & \bfseries 3.17e-3 ± 4.3e-3 \\
IC & Caltech101 5-shot & BiT/50/1 & 46 & 54 & 2.34e-1 ± 6.1e-3 & 4.13e-2 ± 2.1e-3 & 1.61e-2 ± 1.3e-3 & 4.49e-2 ± 2.1e-3 & \bfseries 1.33e-2 ± 2.2e-3 \\
IC & Caltech101 5-shot & MiX/B/16 & 24 & 19 & 2.43e-1 ± 1.2e-2 & 2.43e-1 ± 1.2e-2 & 2.35e-1 ± 1.1e-2 & 1.23e-1 ± 6.0e-3 & \bfseries 3.59e-3 ± 1.9e-3 \\
IC & Caltech101 5-shot & MiX/L/16 & 14 & 13 & 1.38e-1 ± 9.7e-3 & 1.38e-1 ± 9.7e-3 & 1.38e-1 ± 9.7e-3 & 3.19e-2 ± 2.6e-3 & \bfseries 3.19e-2 ± 1.1e-2 \\
IC & Caltech101 5-shot & ViT/B/16 & 38 & 41 & 1.10e-1 ± 6.3e-3 & 1.10e-1 ± 6.3e-3 & 6.02e-2 ± 4.7e-3 & 6.59e-2 ± 4.7e-3 & \bfseries 2.33e-2 ± 6.0e-3 \\
IC & Caltech101 5-shot & ViT/S/16 & 49 & 82 & 1.90e-1 ± 4.7e-3 & 3.82e-2 ± 2.6e-3 & 5.04e-2 ± 2.9e-3 & 4.06e-2 ± 2.7e-3 & \bfseries 2.47e-2 ± 3.8e-3 \\
IC & ImageNet 10-shot & BiT/101/3 & 60 & 118 & 1.27e-1 ± 2.0e-3 & 1.27e-1 ± 2.0e-3 & 7.36e-2 ± 1.1e-3 & 2.13e-2 ± 5.8e-4 & \bfseries 5.95e-3 ± 5.5e-4 \\
IC & ImageNet 10-shot & BiT/50/1 & 68 & 262 & 9.54e-2 ± 7.2e-4 & 9.54e-2 ± 7.2e-4 & \bfseries 5.75e-3 ± 2.0e-4 & 1.77e-2 ± 2.7e-4 & 8.93e-3 ± 2.7e-4 \\
IC & ImageNet 10-shot & MiX/B/16 & 69 & 329 & 9.34e-2 ± 7.9e-4 & 9.34e-2 ± 7.9e-4 & 3.37e-2 ± 2.9e-4 & 1.80e-2 ± 2.7e-4 & \bfseries 5.88e-3 ± 2.5e-4 \\
IC & ImageNet 10-shot & MiX/L/16 & 66 & 249 & 9.83e-2 ± 1.3e-3 & 9.83e-2 ± 1.3e-3 & 9.83e-2 ± 1.3e-3 & 9.48e-3 ± 2.4e-4 & \bfseries 3.81e-3 ± 2.9e-4 \\
IC & ImageNet 10-shot & ViT/B/16 & 67 & 289 & 4.62e-2 ± 7.1e-4 & 4.62e-2 ± 7.1e-4 & 4.62e-2 ± 7.1e-4 & 3.43e-2 ± 4.4e-4 & \bfseries 2.85e-3 ± 2.7e-4 \\
IC & ImageNet 10-shot & ViT/S/16 & 65 & 310 & 4.74e-2 ± 5.6e-4 & 4.74e-2 ± 5.6e-4 & 1.66e-2 ± 2.5e-4 & 1.14e-2 ± 2.4e-4 & \bfseries 1.97e-3 ± 1.4e-4 \\
IC & ImageNet 25-shot & BiT/101/3 & 57 & 100 & 1.42e-1 ± 2.3e-3 & 1.42e-1 ± 2.3e-3 & 6.67e-2 ± 9.1e-4 & 2.18e-2 ± 7.0e-4 & \bfseries 4.86e-3 ± 6.2e-4 \\
IC & ImageNet 25-shot & BiT/50/1 & 68 & 263 & 1.17e-1 ± 9.2e-4 & 1.17e-1 ± 9.2e-4 & \bfseries 4.06e-3 ± 1.7e-4 & 1.70e-2 ± 2.5e-4 & 8.14e-3 ± 2.4e-4 \\
IC & ImageNet 25-shot & MiX/B/16 & 68 & 284 & 9.59e-2 ± 9.3e-4 & 9.59e-2 ± 9.3e-4 & 5.39e-2 ± 4.9e-4 & 1.47e-2 ± 2.7e-4 & \bfseries 2.86e-3 ± 2.3e-4 \\
IC & ImageNet 25-shot & MiX/L/16 & 66 & 226 & 1.03e-1 ± 1.3e-3 & 1.03e-1 ± 1.3e-3 & 1.03e-1 ± 1.3e-3 & 6.09e-3 ± 2.5e-4 & \bfseries 1.94e-3 ± 2.6e-4 \\
IC & ImageNet 25-shot & ViT/B/16 & 67 & 289 & 5.17e-2 ± 8.8e-4 & 5.17e-2 ± 8.8e-4 & 5.17e-2 ± 8.8e-4 & 3.26e-2 ± 5.4e-4 & \bfseries 6.91e-3 ± 4.3e-4 \\
IC & ImageNet 25-shot & ViT/S/16 & 65 & 311 & 5.52e-2 ± 4.4e-4 & 4.12e-2 ± 3.4e-4 & 9.65e-3 ± 2.3e-4 & 1.16e-2 ± 2.2e-4 & \bfseries 3.09e-3 ± 2.4e-4 \\
IC & ImageNet 5-shot & BiT/101/3 & 60 & 124 & 9.24e-2 ± 1.4e-3 & 9.24e-2 ± 1.4e-3 & 9.24e-2 ± 1.4e-3 & 1.01e-2 ± 5.3e-4 & \bfseries 2.55e-3 ± 5.0e-4 \\
IC & ImageNet 5-shot & BiT/50/1 & 69 & 305 & 8.95e-2 ± 6.7e-4 & 8.95e-2 ± 6.7e-4 & 1.53e-2 ± 2.2e-4 & 1.03e-2 ± 2.3e-4 & \bfseries 4.00e-3 ± 2.1e-4 \\
IC & ImageNet 5-shot & MiX/B/16 & 70 & 394 & 9.09e-2 ± 7.2e-4 & 9.09e-2 ± 7.2e-4 & 3.01e-2 ± 2.8e-4 & 1.45e-2 ± 2.5e-4 & \bfseries 3.57e-3 ± 2.3e-4 \\
IC & ImageNet 5-shot & MiX/L/16 & 67 & 240 & 7.99e-2 ± 9.7e-4 & 7.99e-2 ± 9.7e-4 & 7.99e-2 ± 9.7e-4 & 5.66e-3 ± 3.1e-4 & \bfseries 1.63e-3 ± 2.4e-4 \\
IC & ImageNet 5-shot & ViT/B/16 & 68 & 361 & 4.11e-2 ± 6.3e-4 & 4.11e-2 ± 6.3e-4 & 4.11e-2 ± 6.3e-4 & 2.88e-2 ± 3.6e-4 & \bfseries 4.97e-3 ± 2.7e-4 \\
IC & ImageNet 5-shot & ViT/S/16 & 66 & 323 & 4.20e-2 ± 4.1e-4 & 4.20e-2 ± 4.1e-4 & 2.40e-2 ± 2.6e-4 & 1.44e-2 ± 2.2e-4 & \bfseries 3.00e-3 ± 1.7e-4 \\
NMT & upstream test cross-entropy & 28 Enc, 6 Dec & 9 & 1 & 1.71e-1 ± 0 & 5.63e-2 ± 0 & 3.37e-2 ± 0 & 1.50e-2 ± 0 & \bfseries 5.13e-3 ± 0 \\
NMT & upstream test cross-entropy & 6 Enc, 28 Dec & 10 & 1 & 2.34e-1 ± 0 & 5.27e-2 ± 0 & 1.65e-2 ± 0 & 3.21e-2 ± 0 & \bfseries 9.81e-3 ± 0 \\
NMT & upstream test cross-entropy & 6 Enc, 6 Dec & 10 & 1 & 2.62e-1 ± 0 & 3.84e-2 ± 0 & 8.92e-2 ± 0 & \bfseries 1.05e-2 ± 0 & 1.41e-2 ± 0 \\
NMT & upstream test cross-entropy & Dec-only, LM & 10 & 1 & 2.52e-1 ± 0 & 1.03e-2 ± 0 & 3.28e-2 ± 0 & 8.88e-3 ± 0 & \bfseries 2.79e-3 ± 0 \\
NMT & upstream test cross-entropy & Trans-E, LSTM-D & 9 & 1 & 1.90e-1 ± 0 & 1.26e-2 ± 0 & 6.32e-2 ± 0 & 1.31e-2 ± 0 & \bfseries 3.08e-3 ± 0 \\
LM & upstream test cross-entropy& 1.07e+9 Param & 44 & 40 & 1.71e-2 ± 6.0e-4 & 1.02e-3 ± 3.5e-5 & 4.50e-3 ± 5.9e-5 & \bfseries 3.79e-4 ± 4.0e-5 & 8.26e-4 ± 3.2e-5 \\
LM & upstream test cross-entropy& 1.34e+8 Param & 48 & 48 & 1.43e-2 ± 4.8e-4 & 1.33e-3 ± 6.5e-5 & \bfseries 6.46e-4 ± 5.1e-5 & 8.14e-4 ± 5.3e-5 & 8.09e-4 ± 5.5e-5 \\
LM & upstream test cross-entropy& 1.68e+7 Param & 236 & 240 & 6.37e-3 ± 9.4e-5 & \bfseries 3.08e-4 ± 1.3e-5 & 1.24e-3 ± 3.2e-5 & 3.27e-4 ± 1.5e-5 & 4.05e-4 ± 1.8e-5 \\
LM & upstream test cross-entropy& 2.62e+8 Param & 156 & 20 & 1.55e-2 ± 7.2e-4 & 1.01e-3 ± 9.4e-5 & 3.97e-3 ± 1.3e-4 & \bfseries 9.37e-4 ± 9.7e-5 & 1.80e-3 ± 5.6e-5 \\
LM & upstream test cross-entropy& 4.53e+8 Param & 44 & 40 & 1.65e-2 ± 6.6e-4 & 6.47e-4 ± 8.5e-5 & 6.58e-4 ± 6.6e-5 & 8.54e-4 ± 4.7e-5 & \bfseries 5.10e-4 ± 7.7e-5 \\
\end{tabular}
    \caption{
    Extrapolation Results for Each of Every Task from Scaling Laws Benchmark Dataset. Numbers for M1, M2, M3, and M4 obtained via correspondence with authors of \cite{Alabdulmohsi2022revisiting}. Bolded if lowest in row or below 1e-3.
    }
    \label{table:scaling_laws_benchmark_dataset__All}
\end{table}
\FloatBarrier

\subsection{Plots of BNSL Extrapolations}
\label{section:Plots_of_BNSL_Extrapolations}

\FloatBarrier
\begin{figure*}
    \centering

\includegraphics[width=0.245\textwidth]{figures/scaling_laws_benchmark_dataset_plots/birds_5___BiT^50^1.png}
\includegraphics[width=0.245\textwidth]{figures/scaling_laws_benchmark_dataset_plots/birds_5___BiT^101^3.png}
\includegraphics[width=0.245\textwidth]{figures/scaling_laws_benchmark_dataset_plots/birds_5___MiX^B^16.png}
\includegraphics[width=0.245\textwidth]{figures/scaling_laws_benchmark_dataset_plots/birds_5___MiX^L^16.png}
\includegraphics[width=0.245\textwidth]{figures/scaling_laws_benchmark_dataset_plots/birds_5___ViT^B^16.png}
\includegraphics[width=0.245\textwidth]{figures/scaling_laws_benchmark_dataset_plots/birds_5___ViT^S^16.png}
\includegraphics[width=0.245\textwidth]{figures/scaling_laws_benchmark_dataset_plots/birds_10___BiT^50^1.png}
\includegraphics[width=0.245\textwidth]{figures/scaling_laws_benchmark_dataset_plots/birds_10___BiT^101^3.png}
\includegraphics[width=0.245\textwidth]{figures/scaling_laws_benchmark_dataset_plots/birds_10___MiX^B^16.png}
\includegraphics[width=0.245\textwidth]{figures/scaling_laws_benchmark_dataset_plots/birds_10___MiX^L^16.png}
\includegraphics[width=0.245\textwidth]{figures/scaling_laws_benchmark_dataset_plots/birds_10___ViT^B^16.png}
\includegraphics[width=0.245\textwidth]{figures/scaling_laws_benchmark_dataset_plots/birds_10___ViT^S^16.png}
\includegraphics[width=0.245\textwidth]{figures/scaling_laws_benchmark_dataset_plots/birds_25___BiT^50^1.png}
\includegraphics[width=0.245\textwidth]{figures/scaling_laws_benchmark_dataset_plots/birds_25___BiT^101^3.png}
\includegraphics[width=0.245\textwidth]{figures/scaling_laws_benchmark_dataset_plots/birds_25___MiX^B^16.png}
\includegraphics[width=0.245\textwidth]{figures/scaling_laws_benchmark_dataset_plots/birds_25___MiX^L^16.png}
\includegraphics[width=0.245\textwidth]{figures/scaling_laws_benchmark_dataset_plots/birds_25___ViT^B^16.png}
\includegraphics[width=0.245\textwidth]{figures/scaling_laws_benchmark_dataset_plots/birds_25___ViT^S^16.png}

    \caption{
    Birds 200
    }
    \label{fig:scaling_laws_benchmark_dataset__birds}
\end{figure*}


\begin{figure*}
    \centering


\includegraphics[width=0.245\textwidth]{figures/scaling_laws_benchmark_dataset_plots/c100_5___BiT^50^1.png}
\includegraphics[width=0.245\textwidth]{figures/scaling_laws_benchmark_dataset_plots/c100_5___BiT^101^3.png}
\includegraphics[width=0.245\textwidth]{figures/scaling_laws_benchmark_dataset_plots/c100_5___MiX^B^16.png}
\includegraphics[width=0.245\textwidth]{figures/scaling_laws_benchmark_dataset_plots/c100_5___MiX^L^16.png}
\includegraphics[width=0.245\textwidth]{figures/scaling_laws_benchmark_dataset_plots/c100_5___ViT^B^16.png}
\includegraphics[width=0.245\textwidth]{figures/scaling_laws_benchmark_dataset_plots/c100_5___ViT^S^16.png}
\includegraphics[width=0.245\textwidth]{figures/scaling_laws_benchmark_dataset_plots/c100_10___BiT^50^1.png}
\includegraphics[width=0.245\textwidth]{figures/scaling_laws_benchmark_dataset_plots/c100_10___BiT^101^3.png}
\includegraphics[width=0.245\textwidth]{figures/scaling_laws_benchmark_dataset_plots/c100_10___MiX^B^16.png}
\includegraphics[width=0.245\textwidth]{figures/scaling_laws_benchmark_dataset_plots/c100_10___MiX^L^16.png}
\includegraphics[width=0.245\textwidth]{figures/scaling_laws_benchmark_dataset_plots/c100_10___ViT^B^16.png}
\includegraphics[width=0.245\textwidth]{figures/scaling_laws_benchmark_dataset_plots/c100_10___ViT^S^16.png}
\includegraphics[width=0.245\textwidth]{figures/scaling_laws_benchmark_dataset_plots/c100_25___BiT^50^1.png}
\includegraphics[width=0.245\textwidth]{figures/scaling_laws_benchmark_dataset_plots/c100_25___BiT^101^3.png}
\includegraphics[width=0.245\textwidth]{figures/scaling_laws_benchmark_dataset_plots/c100_25___MiX^B^16.png}
\includegraphics[width=0.245\textwidth]{figures/scaling_laws_benchmark_dataset_plots/c100_25___MiX^L^16.png}
\includegraphics[width=0.245\textwidth]{figures/scaling_laws_benchmark_dataset_plots/c100_25___ViT^B^16.png}
\includegraphics[width=0.245\textwidth]{figures/scaling_laws_benchmark_dataset_plots/c100_25___ViT^S^16.png}

    \caption{
    CIFAR-100
    }
    \label{fig:scaling_laws_benchmark_dataset__cifar_100}
\end{figure*}


\begin{figure*}
    \centering

\includegraphics[width=0.245\textwidth]{figures/scaling_laws_benchmark_dataset_plots/caltech_5shot___BiT^50^1.png}
\includegraphics[width=0.245\textwidth]{figures/scaling_laws_benchmark_dataset_plots/caltech_5shot___BiT^101^3.png}
\includegraphics[width=0.245\textwidth]{figures/scaling_laws_benchmark_dataset_plots/caltech_5shot___MiX^B^16.png}
\includegraphics[width=0.245\textwidth]{figures/scaling_laws_benchmark_dataset_plots/caltech_5shot___MiX^L^16.png}
\includegraphics[width=0.245\textwidth]{figures/scaling_laws_benchmark_dataset_plots/caltech_5shot___ViT^B^16.png}
\includegraphics[width=0.245\textwidth]{figures/scaling_laws_benchmark_dataset_plots/caltech_5shot___ViT^S^16.png}
\includegraphics[width=0.245\textwidth]{figures/scaling_laws_benchmark_dataset_plots/caltech_10shot___BiT^50^1.png}
\includegraphics[width=0.245\textwidth]{figures/scaling_laws_benchmark_dataset_plots/caltech_10shot___BiT^101^3.png}
\includegraphics[width=0.245\textwidth]{figures/scaling_laws_benchmark_dataset_plots/caltech_10shot___MiX^B^16.png}
\includegraphics[width=0.245\textwidth]{figures/scaling_laws_benchmark_dataset_plots/caltech_10shot___MiX^L^16.png}
\includegraphics[width=0.245\textwidth]{figures/scaling_laws_benchmark_dataset_plots/caltech_10shot___ViT^B^16.png}
\includegraphics[width=0.245\textwidth]{figures/scaling_laws_benchmark_dataset_plots/caltech_10shot___ViT^S^16.png}
\includegraphics[width=0.245\textwidth]{figures/scaling_laws_benchmark_dataset_plots/caltech_25shot___BiT^50^1.png}
\includegraphics[width=0.245\textwidth]{figures/scaling_laws_benchmark_dataset_plots/caltech_25shot___BiT^101^3.png}
\includegraphics[width=0.245\textwidth]{figures/scaling_laws_benchmark_dataset_plots/caltech_25shot___MiX^B^16.png}
\includegraphics[width=0.245\textwidth]{figures/scaling_laws_benchmark_dataset_plots/caltech_25shot___MiX^L^16.png}
\includegraphics[width=0.245\textwidth]{figures/scaling_laws_benchmark_dataset_plots/caltech_25shot___ViT^B^16.png}
\includegraphics[width=0.245\textwidth]{figures/scaling_laws_benchmark_dataset_plots/caltech_25shot___ViT^S^16.png}

    \caption{
    Caltech101
    }
    \label{fig:scaling_laws_benchmark_dataset__caltech}
\end{figure*}


\begin{figure*}
    \centering

\includegraphics[width=0.245\textwidth]{figures/scaling_laws_benchmark_dataset_plots/few_shot_5___BiT^50^1.png}
\includegraphics[width=0.245\textwidth]{figures/scaling_laws_benchmark_dataset_plots/few_shot_5___BiT^101^3.png}
\includegraphics[width=0.245\textwidth]{figures/scaling_laws_benchmark_dataset_plots/few_shot_5___MiX^B^16.png}
\includegraphics[width=0.245\textwidth]{figures/scaling_laws_benchmark_dataset_plots/few_shot_5___MiX^L^16.png}
\includegraphics[width=0.245\textwidth]{figures/scaling_laws_benchmark_dataset_plots/few_shot_5___ViT^B^16.png}
\includegraphics[width=0.245\textwidth]{figures/scaling_laws_benchmark_dataset_plots/few_shot_5___ViT^S^16.png}
\includegraphics[width=0.245\textwidth]{figures/scaling_laws_benchmark_dataset_plots/few_shot_10___BiT^50^1.png}
\includegraphics[width=0.245\textwidth]{figures/scaling_laws_benchmark_dataset_plots/few_shot_10___BiT^101^3.png}
\includegraphics[width=0.245\textwidth]{figures/scaling_laws_benchmark_dataset_plots/few_shot_10___MiX^B^16.png}
\includegraphics[width=0.245\textwidth]{figures/scaling_laws_benchmark_dataset_plots/few_shot_10___MiX^L^16.png}
\includegraphics[width=0.245\textwidth]{figures/scaling_laws_benchmark_dataset_plots/few_shot_10___ViT^B^16.png}
\includegraphics[width=0.245\textwidth]{figures/scaling_laws_benchmark_dataset_plots/few_shot_10___ViT^S^16.png}
\includegraphics[width=0.245\textwidth]{figures/scaling_laws_benchmark_dataset_plots/few_shot_25___BiT^50^1.png}
\includegraphics[width=0.245\textwidth]{figures/scaling_laws_benchmark_dataset_plots/few_shot_25___BiT^101^3.png}
\includegraphics[width=0.245\textwidth]{figures/scaling_laws_benchmark_dataset_plots/few_shot_25___MiX^B^16.png}
\includegraphics[width=0.245\textwidth]{figures/scaling_laws_benchmark_dataset_plots/few_shot_25___MiX^L^16.png}
\includegraphics[width=0.245\textwidth]{figures/scaling_laws_benchmark_dataset_plots/few_shot_25___ViT^B^16.png}
\includegraphics[width=0.245\textwidth]{figures/scaling_laws_benchmark_dataset_plots/few_shot_25___ViT^S^16.png}

    \caption{
    ImageNet
    }
    \label{fig:scaling_laws_benchmark_dataset__ImageNet}
\end{figure*}

\begin{figure*}
    \centering

\includegraphics[width=0.245\textwidth]{figures/scaling_laws_benchmark_dataset_plots/('date_understanding', '1-shot')___262M.png}
\includegraphics[width=0.245\textwidth]{figures/scaling_laws_benchmark_dataset_plots/('date_understanding', '2-shot')___262M.png}
\includegraphics[width=0.245\textwidth]{figures/scaling_laws_benchmark_dataset_plots/('linguistic_mappings', '1-shot')___262M.png}
\includegraphics[width=0.245\textwidth]{figures/scaling_laws_benchmark_dataset_plots/('linguistic_mappings', '2-shot')___262M.png}
\includegraphics[width=0.245\textwidth]{figures/scaling_laws_benchmark_dataset_plots/('mult_data_wrangling', '1-shot')___262M.png}
\includegraphics[width=0.245\textwidth]{figures/scaling_laws_benchmark_dataset_plots/('mult_data_wrangling', '2-shot')___262M.png}
\includegraphics[width=0.245\textwidth]{figures/scaling_laws_benchmark_dataset_plots/('qa_wikidata', '1-shot')___262M.png}
\includegraphics[width=0.245\textwidth]{figures/scaling_laws_benchmark_dataset_plots/('qa_wikidata', '2-shot')___262M.png}
\includegraphics[width=0.245\textwidth]{figures/scaling_laws_benchmark_dataset_plots/('unit_conversion', '1-shot')___262M.png}
\includegraphics[width=0.245\textwidth]{figures/scaling_laws_benchmark_dataset_plots/('unit_conversion', '2-shot')___262M.png}

    \caption{
    BIG Bench
    }
    \label{fig:scaling_laws_benchmark_dataset__big_bench}
\end{figure*}

\begin{figure*}
    \centering

\includegraphics[width=0.245\textwidth]{figures/scaling_laws_benchmark_dataset_plots/log_perplexity___6 Enc, 6 Dec.png}
\includegraphics[width=0.245\textwidth]{figures/scaling_laws_benchmark_dataset_plots/log_perplexity___6 Enc, 28 Dec.png}
\includegraphics[width=0.245\textwidth]{figures/scaling_laws_benchmark_dataset_plots/log_perplexity___28 Enc, 6 Dec.png}
\includegraphics[width=0.245\textwidth]{figures/scaling_laws_benchmark_dataset_plots/log_perplexity___Decoder-only, Language modeling.png}
\includegraphics[width=0.245\textwidth]{figures/scaling_laws_benchmark_dataset_plots/log_perplexity___Transfomer-Encoder, LSTM-Decoder.png}

    \caption{
    NMT
    }
    \label{fig:scaling_laws_benchmark_dataset__nmt}
\end{figure*}

\begin{figure*}
    \centering


\includegraphics[width=0.245\textwidth]{figures/scaling_laws_benchmark_dataset_plots/validation loss___1.07e+09.png}
\includegraphics[width=0.245\textwidth]{figures/scaling_laws_benchmark_dataset_plots/validation loss___1.34e+08.png}
\includegraphics[width=0.245\textwidth]{figures/scaling_laws_benchmark_dataset_plots/validation loss___1.68e+07.png}
\includegraphics[width=0.245\textwidth]{figures/scaling_laws_benchmark_dataset_plots/validation loss___2.62e+08.png}
\includegraphics[width=0.245\textwidth]{figures/scaling_laws_benchmark_dataset_plots/validation loss___4.53e+08.png}

    \caption{
    Language Modeling
    }
    \label{fig:scaling_laws_benchmark_dataset__language_modeling}
\end{figure*}

\FloatBarrier
